# Supplementary material for: Dordis: Efficient Federated Learning with Dropout-Resilient Differential Privacy
Source: arXiv:2209.12528 source file (2023-11-10)
Supplement: Supplementary file 1 [file complexity.tex]

%!TEX root = ../main.tex
\section{Noise Enforcement Complexity Analysis}
~\label{sec:appendix_complexity}

\vspace*{-0.15in}

We first evaluate the complexity of \texttt{XNoise-Prec} (\cref{sec:enforcement_add}).
All calculations below assume a single server and $\lvert S \rvert$ users, where $\lvert D \rvert = O(\lvert S \rvert)$ clients drop out after being sampled.
We also use $d$ to denote the number of parameters in a model.
We ignore the cost of the used public key infrastructure but stress that including its cost does not change any of the asymptotics.

For a sampled client, its computational cost
stems from (1) generating noise components, which is $O(\lvert S \rvert)$,
(2) adding the noise components to its update, which is $O(d\lvert S \rvert)$
where $d$ is the model size, measured by the number of model parameters, and
(3) creating secret shares for the used PRG seeds, which is $O
(\lvert S \rvert^3)$. Together, the computational complexity 
is $O(d\lvert S \rvert + \lvert S \rvert^3)$.
Concerning the communication cost, it stems from (1) uploading the needed seeds 
for noise removal, which is $O(\lvert S \rvert)$, and, if necessary, (2) 
uploading the secret shares for recovering the other clients' missing seeds, 
which is $O(\lvert S \rvert^2)$.
The overall communication complexity is hence $O(\lvert S \rvert^2)$.

For the server, its computational cost stems from (1) recovering the missing
seeds, if any, using the optimized reconstruction technique given in~\cite
{bonawitz2017practical}, which is $O(\lvert S \rvert^3)$, and (2) generating
excessive noise components using the PRG seeds and removing them, which is $O
(d \lvert S \rvert^2)$. Thus, the overall computational complexity is $O
(\lvert S \rvert^3 + d \lvert S \rvert^2)$. As for the server's
communication cost, it stems from (1) receiving PRG seeds from surviving clients,
which is $O(\lvert S \rvert^2)$, and (2) receiving secret
shares for recovering the missing seeds (if any), which is
$O(\lvert S \rvert^3)$. Overall, the  communication complexity is $O
(\lvert S \rvert^3)$.

The analysis of \texttt{XNoise-Appr} (\cref{sec:enforcement_scalability}) is almost the same as the above, except that each client generates $O(\log \lvert S \rvert)$ noise components instead of $O(\lvert S \rvert)$. We thus omit it for brevity.
