# Supplementary material for: Dordis: Efficient Federated Learning with Dropout-Resilient Differential Privacy
Source: arXiv:2209.12528 source file (2023-11-10)
Supplement: Supplementary file 2 [file secagg.tex]

%!TEX root = ../main.tex
\section{The SecAgg protocol}~\label{sec:appendix_secagg}

\vspace*{-0.15in}

\PHB{Technical Details.} Here we provide a detailed description of how SecAgg~\cite{bonawitz2017practical} works under the semi-honest adversary.
As depicted in Fig.~\ref{fig:secagg}, the protocol consists of four communication rounds.

\begin{figure}[t]
    \centering
    \includegraphics[width=1.0\columnwidth]{./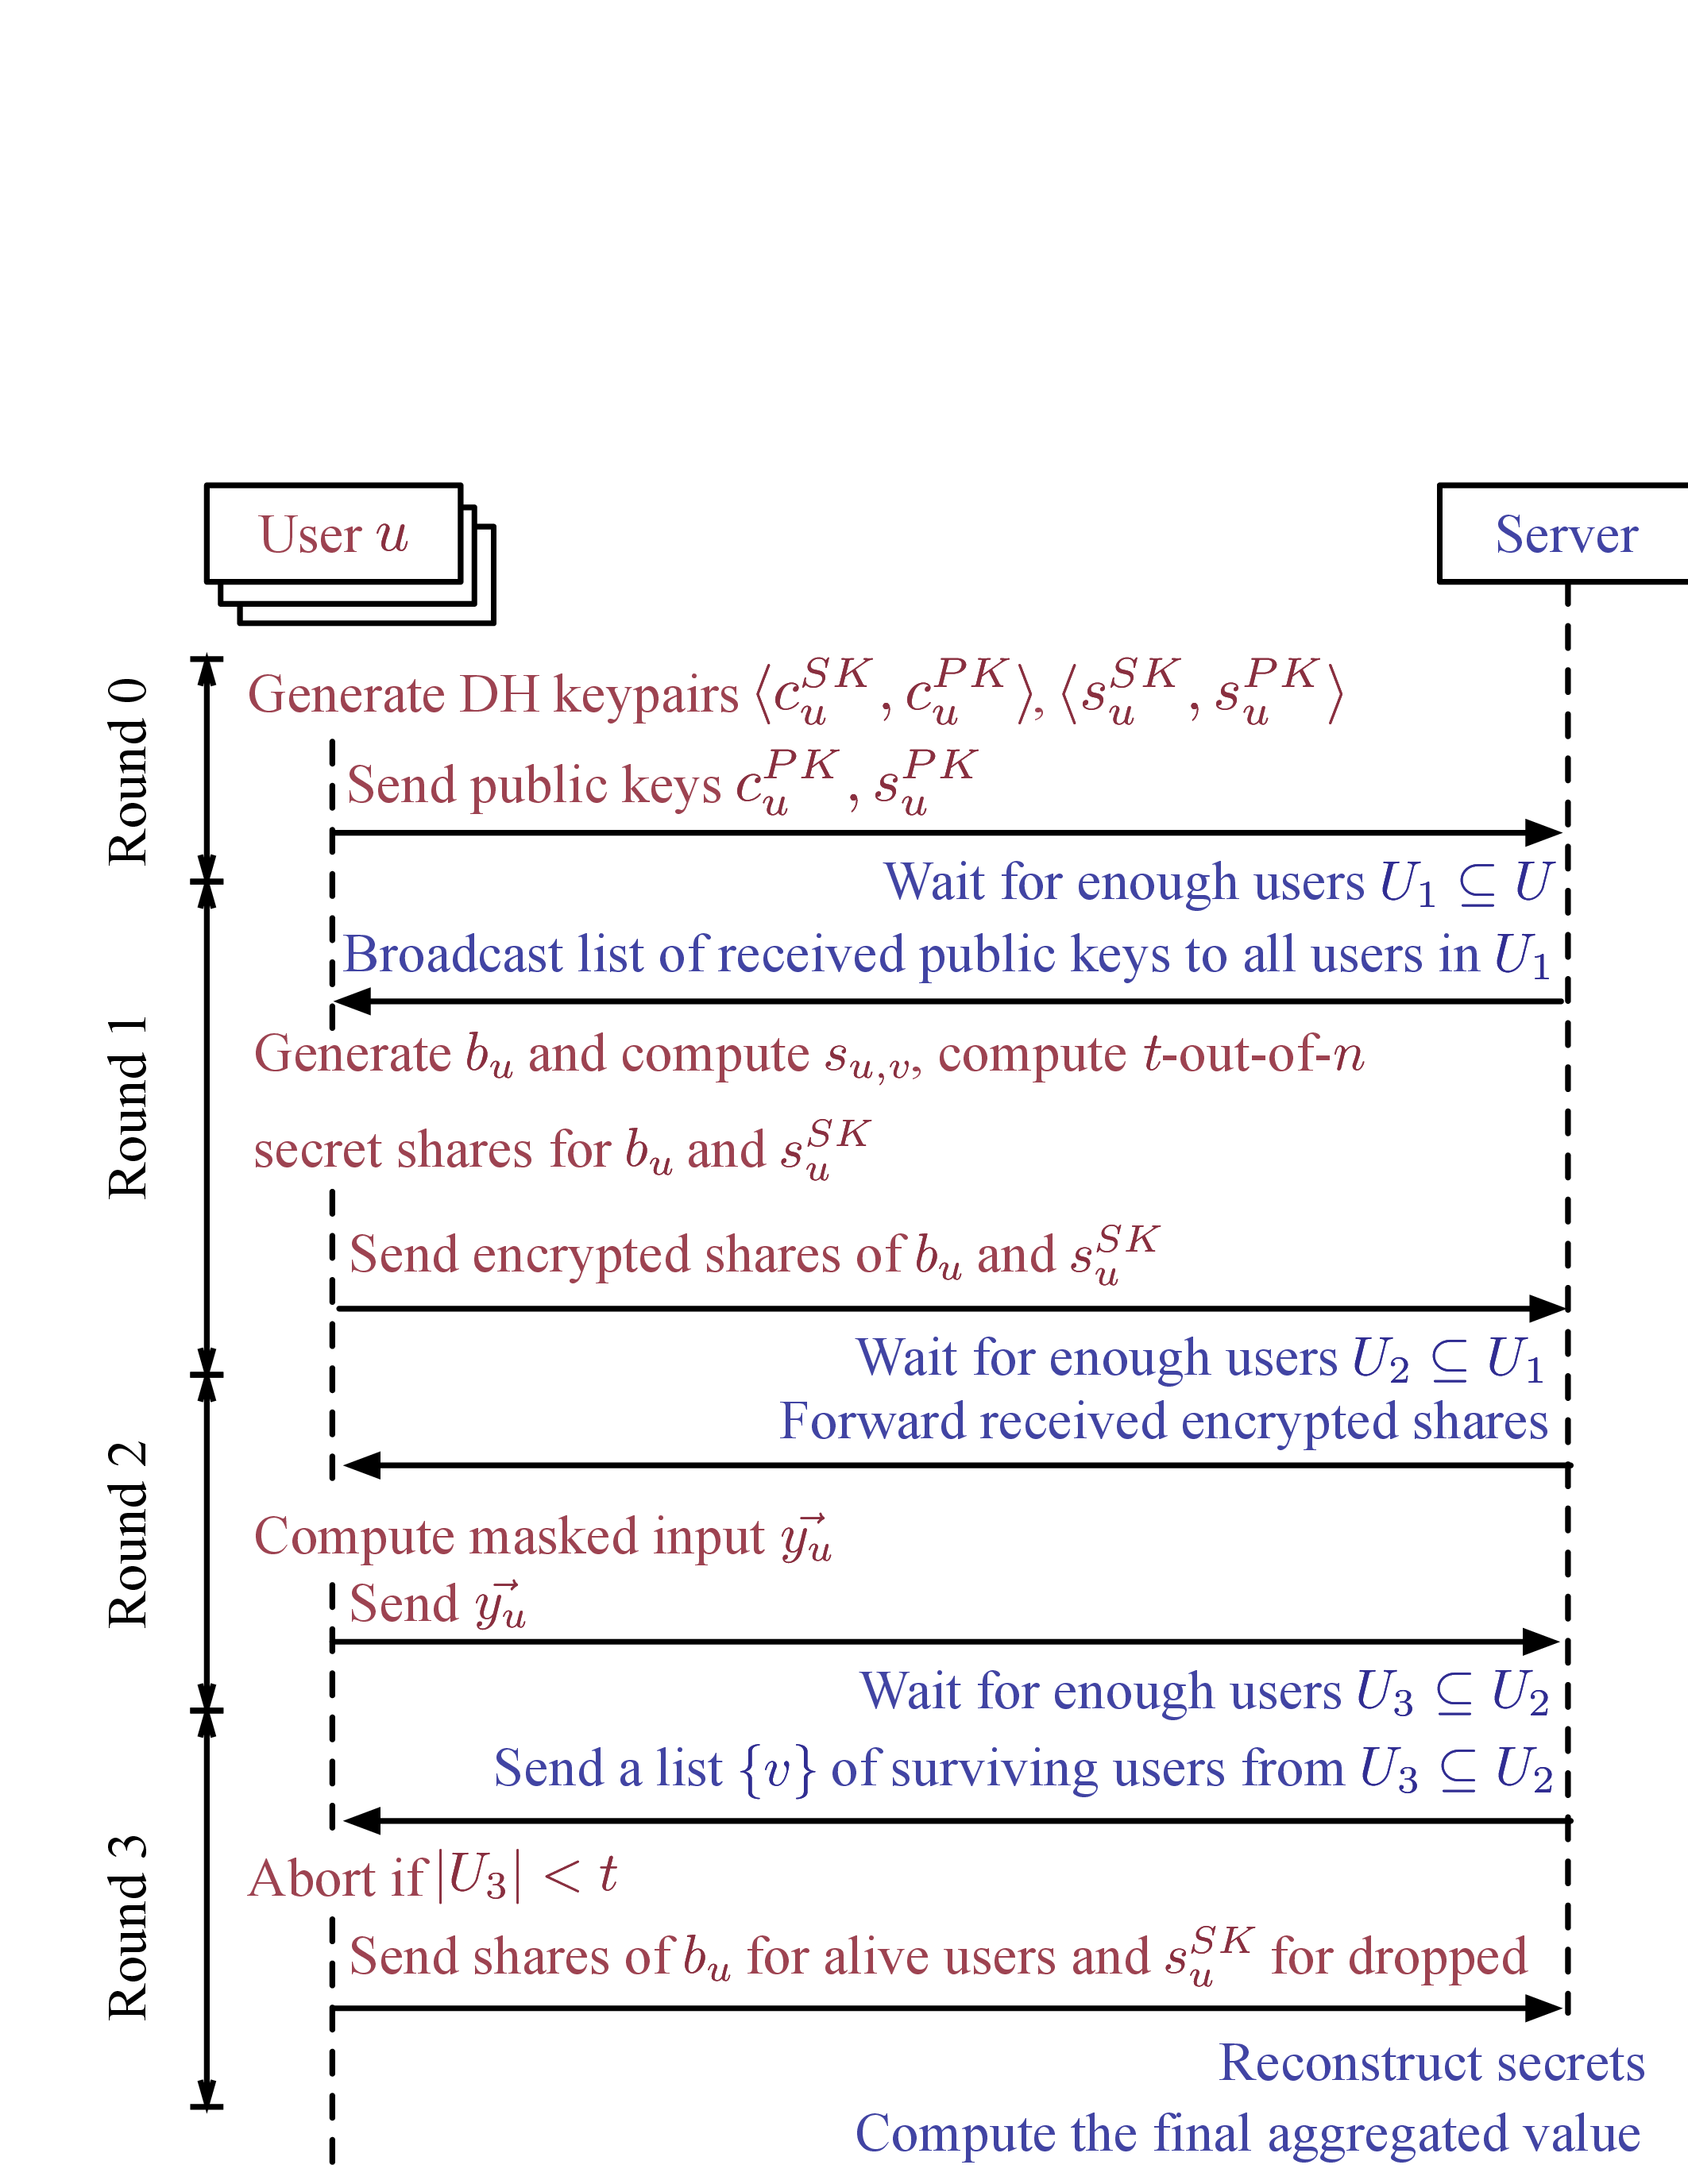}
    \caption{SecAgg's protocol in the semi-honest threat model~\cite{bonawitz2017practical}.}
    \label{fig:secagg}
\end{figure}

\begin{itemize}
    \item \textit{Round 0 (Advertise Keys)}: each client $u \in U$ generates key pairs $\langle c_u^{SK}, c_u^{PK} \rangle$, $\langle s_u^{SK}, s_u^{PK} \rangle$ and sends $(c_u^{PK}, s_u^{PK})$ to all of her neighbors with the relaying help of the server.
    \item \textit{Round 1 (Share Keys)}: each of the alive clients $u \in U_1 \subseteq U$ runs the Diffie-Hellman key agreement protocol~\cite{merkle1978secure} that derives a shared random key $s_{u, v} = \mathcal{KA}.Agree(s_u^{SK}, s_v^{PK})$ for every other client $v \in U_1$.\footnote{Note that $\mathcal{KA}.Agree(\cdot, \cdot)$ is symmetric and thus $s_{u, v} = s_{v, u}$}
    Client $u$ also randomly samples a seed $b_u$, and securely shares $s_u^{SK}$ and $b_u$ to each of the other client $v$'s by sending it the respective $t$-out-of-$n$ shares encrypted using the corresponding agreed key $\mathcal{KA}.Agree(c_u^{SK}, c_v^{PK})$'s.
    \item \textit{Round 2 (Masked Input Collection)}: each surviving client $u \in U_2$ prepares a pairwise mask $\vec{m_{u, v}} = PRG(s_{u, v})$ derived from shared keys with each of the other client $v$'s. She also generates a self mask $\vec{r_{u}}=PRG(b_u)$, masks her vector input $\vec{x_u}$ in the following manner and then sends the masked input $\vec{y_u}$ to the server:
    \begin{align}
        \vec{y_u} = \vec{x_u}+\vec{r_u}-\sum_{v<u, v\in U_2} \vec{m_{u, v}} + \sum_{v>u, v\in U_2} \vec{m_{u, v}}.
        \label{eq:secagg_client}
    \end{align}
    \item \textit{Round 3 (Unmasking)}: summing up masked inputs submitted by surviving clients $U_3$, the server obtains:
    \begin{align}
        \sum_{u \in U_3} \vec{x_u} + \underbrace{\sum_{u \in U_3} \vec{r_u}}_{A} + \underbrace{\sum_{u \in U_2/U_3} (\sum_{v < u, v \in U_3} \vec{m_{u, v}} - \sum_{v > u, v \in U_3} \vec{m_{u, v}})}_{B}.
        \label{eq:secagg_server}
    \end{align}
    Then, to remove part $A$, for each surviving client $u \in U_3$, the server compute $\vec{r_u}$ by reconstructing $b_u$ with over $t$ shares of it collected from surviving clients $U_4$. Similarly, to remove part $B$, for each dropped clients $u \in U_2/U_3$, the server reconstructs its secret key $c_u^{SK}$ by collecting over $t$ shares of it from $U_4$. Together with the public keys of $v$'s from $U_2/\{u\}$ to reconstruct $s_{u, v}$'s, the server finally computes and removes all the related $\vec{m_{u, v}}$'s.
\end{itemize}

\PHM{Source of Complexity.}
We now pinpoint two main sources of SecAgg's inefficiency (\cref{sec:background_prior}).
The first source is the use of Shamir's $t$-out-of-$n$ \textit{secret sharing} scheme~\cite{shamir1979share} (Round 1).
It is employed to gain resilience against client dropout, as it allows a secret to be split and shared to $n$ clients so that any $t$ clients can provide enough information to reconstruct it.
For a client, generating Shamir's $t$-out-of-$n$ secret takes $O(n^2)$ time, yielding a quadratic computation overhead w.r.t. the number of sampled clients ($O(\lvert U_1 \rvert^2)$).
The second source is the design of \textit{pairwise masking}, where each client adds a pairwise mask (of the same length $d$ as the model) to her update for each of the other alive clients (Round 2), and the server needs to unmask these masks for each dropped client (Round 3).
This helps tolerate colluding parties, as the pairwise masks between any two benign clients will be concealed from the adversary. However, it induces quadratic computation overhead to both clients ($O(d \lvert U_2 \rvert^2)$) and the server ($O(d \lvert U_3 \rvert^2)$).

% \PHM{Incentive of Correct Dropout report.} When unmasking the sum (Round 3), for each participating client $i\in U_2$, the server either demands secrets to reconstruct $\vec{r_i}$ if the client remains in $U_3$, or those to reconstruct $\vec{m_{i, j}}$ if the client drops. Sending misleading reports about the dropout outcome to clients, e.g., stating a dropped client is still alive, will make the unmasking impossible and result in a masked sum that is indistinguishable from a random number. As for FL training, this will lead to a significant model quality degradation and call for abortion of the federation, from which the server cannot benefit at all. Hence, the server has an incentive to faithfully report dropout outcome ($\lvert U_2/U_3 \rvert$) to alive clients for every round, which \system{} can rely on for noise enforcement (\cref{sec:enforcement_add}).
